# Supplementary material for: Learning to Expand Audience via Meta Hybrid Experts and Critics for Recommendation and Advertising
Source: arXiv:2105.14688 source file (2021-05-31)
Supplement: Supplementary file 1 [file Appendix.tex]

\setcounter{section}{0}
\section{Appendix}
\subsection{Data Collection and Privacy Protection}

The private dataset is collected from "Top Stories" of WeChat. This is a dataset of content promotion in recommender systems. Each task is a content marketing campaign that consists of several contents (items), lots of seed users, and non-seed users. All the campaigns occur in three days in January, 2021. In order to comply with the user privacy and data protection regulation for each user, multiple approaches have been taken in the data processing step, which includes but are not limited to: personally identifiable information (PII) encrypted with salted MD5, data sampling, etc. By doing so, no original data could be restored and the statistics in this manuscript do not represent any real business status. Thus, the private industry dataset (WeChat Look-alike Dataset) does not involve user privacy. 

\subsection{More Experimental Details} For the one-stage baselines LR and MLP\_one-stage, we directly train a customized model (LR and MLP) for a certain campaign without any pre-training. For the MLP+emb, the embedding layer is shared by all campaign tasks and pre-trained on existing campaigns. For a new campaign, based on the pre-trained embeddings, we train a customized model. For Pinterest and Hubble, we mainly follow the original methods. For the MLP+pre-training, both the embedding layer and the network (MLP) are pre-trained on the existing campaigns, and we fine-tune the pre-trained general model for a new campaign. For the Shared-Bottom+pre-training and MMoE+pre-training, the bottom networks are pre-trained on the existing campaigns. Then, we train a customized head and fine-tune the bottom network and embeddings for each new campaign. For MetaHeac and MMoE+pre-training, the number of experts and critics are tuned in [3, 10]. By grid search, we set experts of 8 and critics of 5 for MetaHeac on Tencent Look-alike Dataset. Besides, we set experts of 8 and critics of 3 for MetaHeac on WeChat Look-alike Dataset. By grid search, the number of experts is set as 8 for MMoE+pre-training. For a fair comparison, the number of layers is the same in all methods. The MLP\_one-stage, MLP+emb, Hubble, and MLP+pre-training utilize three layers of MLP (units 64, 64, 1) as customized models. For the Shared-Bottom+pre-training, MMoE+pre-training, and MetaHeac, the layers of the bottom/expert (units 64, 64) and head/critic (unit 1) are similar to the MLP-based methods above. 

To reproduce the results, \textbf{the code for the public Tencent Look-alike Dataset has been available at \url{https://github.com/easezyc/MetaHeac}}.
